# Supplementary material for: Adaptive Graph Pruning with Sudden-Events Evaluation for Traffic Prediction using Online Semi-Decentralized ST-GNNs
Source: arXiv:2512.17352 source file (2025-12-19)
Supplement: Supplementary file 1 [file 6_appendix.tex]

\appendices
\section{\break Footnotes}
Number footnotes separately in superscript numbers.\footnote{It is recommended that footnotes be avoided (except for
the unnumbered footnote with the receipt date on the first page). Instead,
try to integrate the footnote information into the text.} Place the actual
footnote at the bottom of the column in which it is cited; do not put
footnotes in the reference list (endnotes). Use letters for table footnotes
(see Table \ref{table}).

\section{\break Submitting Your Paper for Review}

\subsection{Final Stage}
When your article is accepted, you can submit the final files, including figures, tables, and photos, per the journal's guidelines through the submission system used to submit the articlle.
 You may use \emph{Zip} for large files, or compress files using \emph{Compress, Pkzip, Stuffit,} or \emph{Gzip.}

In addition, designate one author as the ``corresponding author.'' This is the author to
whom proofs of the paper will be sent. Proofs are sent to the corresponding
author only.

\subsection{Review Stage Using IEEE Author Portal}
Article contributions to IEEE Access should be submitted electronically on the IEEE Author Portal. For more information, please visit
\underline{https://ieeeaccess.ieee.org/}.

Along with other information, you will be asked to select the subject from a
pull-down list. There are various steps to the
submission process; you must complete all steps for a complete submission.
At the end of each step you must click ``Save and Continue''; just uploading
the paper is not sufficient. After the last step, you should see a
confirmation that the submission is complete. You should also receive an
e-mail confirmation. For inquiries regarding the submission of your article, please contact ieeeaccess@ieee.org.

The manuscript should be prepared in a double column, single-spaced format using a required IEEE Access template.
A Word or LaTeX file and a PDF file are both required upon submission in the IEEE Author Portal.

\subsection{Final Stage Using IEEE Author Portal}
Upon acceptance, you will receive an email with specific instructions

Designate the author who submitted the manuscript on
IEEE Author Portal as the ``corresponding author.'' This is the only
author to whom proofs of the paper will be sent.

\subsection{Copyright Form}
Authors must submit an electronic IEEE Copyright Form (eCF) upon submitting
their final manuscript files. You can access the eCF system through your
manuscript submission system or through the Author Gateway. You are
responsible for obtaining any necessary approvals and/or security
clearances. For additional information on intellectual property rights,
visit the IEEE Intellectual Property Rights department web page at
\underline{http://www.ieee.org/publications\_standards/publications/}\break\underline{rights/index.html}.

\section{\break IEEE Publishing Policy}
The general IEEE policy requires that authors should only submit original
work that has neither appeared elsewhere for publication, nor is under
review for another refereed publication. The submitting author must disclose
all prior publication(s) and current submissions when submitting a
manuscript. Do not publish ``preliminary'' data or results. To avoid any delays in
publication, please be sure to follow these instructions.  Final
submissions should include source files of your accepted manuscript, high
quality graphic files, and a formatted pdf file. If you have any questions
regarding the final submission process, please contact the administrative
contact for the journal.
author is responsible for obtaining agreement of all coauthors and any
consent required from employers or sponsors before submitting an article.

The IEEE Access Editorial Office does not publish conference
records or proceedings, but can publish articles related to conferences that
have undergone rigorous peer review. Minimally, two reviews are required for
every article submitted for peer review.

\section{\break Publication Principles}
Authors should consider the following points:

\begin{enumerate}
\item Technical papers submitted for publication must advance the state of knowledge and must cite relevant prior work.
\item The length of a submitted paper should be commensurate with the importance, or appropriate to the complexity, of the work. For example, an obvious extension of previously published work might not be appropriate for publication or might be adequately treated in just a few pages.
\item Authors must convince both peer reviewers and the editors of the scientific and technical merit of a paper; the standards of proof are higher when extraordinary or unexpected results are reported.
\item Because replication is required for scientific progress, papers submitted for publication must provide sufficient information to allow readers to perform similar experiments or calculations and
use the reported results. Although not everything need be disclosed, a paper
must contain new, useable, and fully described information. For example, a
specimen's chemical composition need not be reported if the main purpose of
a paper is to introduce a new measurement technique. Authors should expect
to be challenged by reviewers if the results are not supported by adequate
data and critical details.
\item Papers that describe ongoing work or announce the latest technical achievement, which are suitable for presentation at a professional conference, may not be appropriate for publication.
\end{enumerate}

\section{\break Reference Examples}

\begin{itemize}

\item \emph{Basic format for books:}\\
J. K. Author, ``Title of chapter in the book,'' in \emph{Title of His Published Book, x}th ed. City of Publisher, (only U.S. State), Country: Abbrev. of Publisher, year, ch. $x$, sec. $x$, pp. \emph{xxx--xxx.}\\
See \cite{b1,b2}.

\item \emph{Basic format for periodicals:}\\
J. K. Author, ``Name of paper,'' \emph{Abbrev. Title of Periodical}, vol. \emph{x, no}. $x, $pp\emph{. xxx--xxx, }Abbrev. Month, year, DOI. 10.1109.\emph{XXX}.123456.\\
See \cite{b3}--\cite{b5}.

\item \emph{Basic format for reports:}\\
J. K. Author, ``Title of report,'' Abbrev. Name of Co., City of Co., Abbrev. State, Country, Rep. \emph{xxx}, year.\\
See \cite{b6,b7}.

\item \emph{Basic format for handbooks:}\\
\emph{Name of Manual/Handbook, x} ed., Abbrev. Name of Co., City of Co., Abbrev. State, Country, year, pp. \emph{xxx--xxx.}\\
See \cite{b8,b9}.

\item \emph{Basic format for books (when available online):}\\
J. K. Author, ``Title of chapter in the book,'' in \emph{Title of
Published Book}, $x$th ed. City of Publisher, State, Country: Abbrev.
of Publisher, year, ch. $x$, sec. $x$, pp. \emph{xxx--xxx}. [Online].
Available: \underline{http://www.web.com}\\
See \cite{b10}--\cite{b13}.

\item \emph{Basic format for journals (when available online):}\\
J. K. Author, ``Name of paper,'' \emph{Abbrev. Title of Periodical}, vol. $x$, no. $x$, pp. \emph{xxx--xxx}, Abbrev. Month, year. Accessed on: Month, Day, year, DOI: 10.1109.\emph{XXX}.123456, [Online].\\
See \cite{b14}--\cite{b16}.

\item \emph{Basic format for papers presented at conferences (when available online): }\\
J.K. Author. (year, month). Title. presented at abbrev. conference title. [Type of Medium]. Available: site/path/file\\
See \cite{b17}.

\item \emph{Basic format for reports and handbooks (when available online):}\\
J. K. Author. ``Title of report,'' Company. City, State, Country. Rep. no., (optional: vol./issue), Date. [Online] Available: site/path/file\\
See \cite{b18,b19}.

\item \emph{Basic format for computer programs and electronic documents (when available online): }\\
Legislative body. Number of Congress, Session. (year, month day). \emph{Number of bill or resolution}, \emph{Title}. [Type of medium]. Available: site/path/file\\
See \cite{b20}.

\item \emph{Basic format for patents (when available online):}\\
Name of the invention, by inventor's name. (year, month day). Patent Number [Type of medium]. Available: site/path/file\\
See \cite{b21}.

\item \emph{Basic format}\emph{for conference proceedings (published):}\\
J. K. Author, ``Title of paper,'' in \emph{Abbreviated Name of Conf.}, City of Conf., Abbrev. State (if given), Country, year, pp. \emph{xxxxxx.}\\
See \cite{b22}.

\item \emph{Example for papers presented at conferences (unpublished):}\\
See \cite{b23}.

\item \emph{Basic format for patents}$:$\\
J. K. Author, ``Title of patent,'' U.S. Patent \emph{x xxx xxx}, Abbrev. Month, day, year.\\
See \cite{b24}.

\item \emph{Basic format for theses (M.S.) and dissertations (Ph.D.):}
\begin{enumerate}
\item J. K. Author, ``Title of thesis,'' M.S. thesis, Abbrev. Dept., Abbrev. Univ., City of Univ., Abbrev. State, year.
\item J. K. Author, ``Title of dissertation,'' Ph.D. dissertation, Abbrev. Dept., Abbrev. Univ., City of Univ., Abbrev. State, year.
\end{enumerate}
See \cite{b25,b26}.

\item \emph{Basic format for the most common types of unpublished references:}
\begin{enumerate}
\item J. K. Author, private communication, Abbrev. Month, year.
\item J. K. Author, ``Title of paper,'' unpublished.
\item J. K. Author, ``Title of paper,'' to be published.
\end{enumerate}
See \cite{b27}--\cite{b29}.

\item \emph{Basic formats for standards:}
\begin{enumerate}
\item \emph{Title of Standard}, Standard number, date.
\item \emph{Title of Standard}, Standard number, Corporate author, location, date.
\end{enumerate}
See \cite{b30,b31}.

\item \emph{Article number in~reference examples:}\\
See \cite{b32,b33}.

\item \emph{Example when using et al.:}\\
See \cite{b34}.

\end{itemize}
